# Supplementary material for: Graph Theorem for Chiral Exact Flat Bands at Charge Neutrality
Source: arXiv:2312.12607 ancillary file (2023-12-19)
Supplement: Supplementary file 1 [file SM.pdf]

**Supplementary Material –**
**"Graph Theorem for Chiral Exact Flat Bands at Charge Neutrality"**

Gurjyot Sethi[1*], Bowen Xia[1*], Dongwook Kim[1], Hang Liu[2,3], Xiaoyin Li[1], and Feng Liu[1]

[1]Department of Materials Science & Engineering, University of Utah, Salt Lake City, UT, 84112
[2]Songshan Lake Materials Laboratory, Dongguan, Guangdong 523808, People's Republic of China
[3]Beijing National Laboratory for Condensed Matter Physics and Institute of Physics, Chinese Academy of Sciences, Beijing 100190, People's Republic of China

## I. Incidence matrices and their correspondence to square-root models

For every graph one can construct an incidence matrix which shows the relationship between the vertices and edges of a graph [1]. This matrix has dimensions $m \times n$, $m$ being the number of edges in the graph and $n$ being the number of vertices and has a matrix element 1 between every vertex and edge that touches each other. For example, in case of honeycomb lattice (illustrated in Fig. S1(a)), if we consider a unit cell in real space, there are 3 independent edges and 2 independent vertices which leads to an incidence matrix,

$$M = \begin{matrix} e/v \\ e_1 \\ e_2 \\ e_3 \end{matrix} \begin{matrix} v_1 \quad v_2 \\ \begin{bmatrix} 1 & 1 \\ 1 & 1 \\ 1 & 1 \end{bmatrix} \end{matrix}.$$

If the lattice is infinite, i.e., periodic, we can use Bloch's theorem to write this matrix in reciprocal space as,

$$M_k = \begin{matrix} e/v \\ e_1 \\ e_2 \\ e_3 \end{matrix} \begin{matrix} v_1 \quad\quad v_2 \\ \begin{bmatrix} 1 & 1 \\ e^{ik.a_1} & 1 \\ e^{ik.a_2} & 1 \end{bmatrix} \end{matrix}.$$

The use of such incidence matrices is very crucial in explaining the lower-bound of the eigenvalues of $A_{L(X)}$, since there exists a graph theorem [2] which states,

$$MM^T = D_X + A_X \,; M^T M = A_{L(X)} + 2I.$$

For honeycomb lattice graph, $D_X = 3I$. Using the incidence matrices, one can further show that the eigen spectra of $A_{L(X)}$ is given by,

$$\sigma\big(A_{L(X)}\big) = \{-2\}^{m-n} \cup \{-2 + \sigma^*(D_X + A_X)\},$$

where $\sigma(A)$ is the set of eigenvalues of matrix A. We refer the readers to Section IV in [3] and references therein for detailed proof. Note that the multiplicity of eigenvalue $-2$ is $m - n$, and the set $\sigma^*(D_X + A_X)$ consists of positive eigenvalues, which shows that the lower bound of the eigenvalues of $A_{L(X)}$ is $-2$. We would like to mention that the eigen spectra relation presented above has a missing factor of $+\eta$ in the multiplicity of $-2$ compared with the expression given in [3] where it was derived for finite graphs. For graphs with translation symmetry or infinite graphs, the extra factor is removed due to double

counting. Clearly if $m > n$, and the graph is periodic, the multiplicity of eigenvalue $-2$ would be infinite. On the other hand, if $m = n$, there won't be such an eigenvalue.

Recently, there has been an increasing interest in the topological square-root tight binding models [4,5,6]. The square root procedure involves considering "mediating sites" between the sites of original lattice that have non-zero hopping between them. In the new composite lattice, hopping is allowed only between the original sites and the mediating sites, rendering the model its chiral symmetry. As an example, consider a honeycomb (H) lattice. The square-root procedure would lead a composite lattice ($S(H)$) shown in Fig. S1(b). The tight-binding Hamiltonian is then given by,

$$\begin{array}{ccc} \text{basis} & \{\text{org.}\} & \{\text{med.}\} \\ H_{S(H)} = \{\text{org.}\} & \multicolumn{2}{c}{\begin{bmatrix} 0_{2\times2} & tM_k \\ tM_k^\dagger & 0_{3\times3} \end{bmatrix}} \\ \{\text{med.}\} & & \end{array},$$

where $0_{y\times y}$ is the null matrix of dimensions $y \times y$, basis set $\{\text{org.}\}$ ($\{\text{med.}\}$) contains 2 (3) original (mediating) sites, and $M_k^\dagger$ is given by,

$$M_k^\dagger = \begin{bmatrix} 1 & 1 \\ e^{ik.a_1} & 1 \\ e^{ik.a_2} & 1 \end{bmatrix}$$

which is exactly the incidence matrix of a honeycomb lattice graph as described above. Hence, there exists a very strong correspondence between the line-graph theorem and the properties of square root lattices. Using the incidence matrix graph theorem, one can also easily notice that the square of $H_{S(H)}$ is given by,

$$H_{S(H)}^2 = \begin{bmatrix} H_H + 3I & 0_{2\times3} \\ 0_{3\times2} & H_{L(H)} + 2I \end{bmatrix},$$

where $H_H$ is the tight binding Hamiltonian of honeycomb lattice, $H_{L(H)}$ is the Hamiltonian of its line-graph (Kagome lattice), and I is the identity matrix. Since the eigenvalues of $H_{S(H)}^2$ are non-negative, there exists a lower bound of 0 for the eigenvalues of $H_{L(H)} + 2I$ or of $-2$ for those of $H_{L(H)}$.

## II. Tight-binding Hamiltonian matrices:

In this section we explicitly present the Hamiltonian matrices for the cases studied in the main text. We use unit-cell gauge under which the Hamiltonian in momentum space satisfies the condition $H(k + G_i) = H(k)$ with $G_i$ being the reciprocal lattice vector. In this gauge the construction of bipartite double cover matrices is quite transparent. One can also use the atomic gauge which gives same results. In the following, t refers to the tight-binding hopping integral between atomic sites/orbitals corresponding to the edges of respective graph based on which the lattice is constructed. For example, in the case of Kagome lattice, t represents the first nearest neighbor hopping integral, while in the case of Kagome-3 lattice, all the first and second, and some of the third nearest-neighbors have the same hopping integral t (Fig. 4). This is because these physical lattices are based on abstract mathematical graphs where the adjacency matrix elements are always 1 whenever the two vertices are connected by an edge irrespective of the edge distance. This is another very crucial reason why we need orbital design principle to find physical real materials where these unphysical hopping constraints can be removed via orbital hybridization and symmetry [7].

a) Kagome lattice (without spin-orbit coupling, spinless) –

$$H(L(H)) = \begin{bmatrix} c_1^{\dagger} & c_2^{\dagger} & c_3^{\dagger} \end{bmatrix} \times \begin{bmatrix} 0 & t(1+e^{-ik.a_1}) & t(1+e^{-ik.(a_1+a_2)}) \\ t(1+e^{ik.a_1}) & 0 & t(1+e^{-ik.a_2}) \\ t(1+e^{ik.(a_1+a_2)}) & t(1+e^{ik.a_2}) & 0 \end{bmatrix} \times \begin{bmatrix} c_1 \\ c_2 \\ c_3 \end{bmatrix}$$

where k is the reciprocal lattice momenta and $a_i$'s are unit-cell vectors depicted in Fig. 2(a). The basis set consists of three atomic sites labelled in Fig. 2(a).

b) Kagome lattice (with spin-orbit coupling, spinful) –

$$\begin{array}{cccccc} c_{1\downarrow}^{\dagger} & c_{2\downarrow}^{\dagger} & c_{3\downarrow}^{\dagger} & c_{1\uparrow}^{\dagger} & c_{2\uparrow}^{\dagger} & c_{3\uparrow}^{\dagger} \end{array}$$
$$\begin{bmatrix} 0 & (t-i\lambda)(1+e^{-ik.a_1}) & (t+i\lambda)(1+e^{-ik.(a_1+a_2)}) & 0 & 0 & 0 \\ (t+i\lambda)(1+e^{ik.a_1}) & 0 & (t-i\lambda)(1+e^{-ik.a_2}) & 0 & 0 & 0 \\ (t-i\lambda)(1+e^{ik.(a_1+a_2)}) & (t+i\lambda)(1+e^{ik.a_2}) & 0 & 0 & 0 & 0 \\ 0 & 0 & 0 & 0 & (t+i\lambda)(1+e^{-ik.a_1}) & (t-i\lambda)(1+e^{-ik.(a_1+a_2)}) \\ 0 & 0 & 0 & (t-i\lambda)(1+e^{ik.a_1}) & 0 & (t+i\lambda)(1+e^{-ik.a_2}) \\ 0 & 0 & 0 & (t+i\lambda)(1+e^{ik.(a_1+a_2)}) & (t-i\lambda)(1+e^{ik.a_2}) & 0 \end{bmatrix}$$

where the notations used are same as defined in a) with the addition of SOC represented by λ. Also, note that there are no matrix elements between spin-up and spin-down states. We use this Hamiltonian to construct a finite lattice in y-direction to check for the presence of edge states. As can be seen from Fig. S2(a), the clear presence of edge states confirms the stable or strong topology of Kagome quasi-FB when SOC is included. In contrast, fragile topological bands have gapless edge states only under twisted boundary conditions [8].

c) Bipartite double cover of Kagome lattice (without SOC, spinless) –

$$\begin{array}{cccccc} c_{1,D}^{\dagger} & c_{2,D}^{\dagger} & c_{3,D}^{\dagger} & c_{1,L}^{\dagger} & c_{2,L}^{\dagger} & c_{3,L}^{\dagger} \end{array}$$
$$\begin{bmatrix} 0 & 0 & 0 & t_0 & t(1+e^{-ik.a_1}) & t(1+e^{-ik.(a_1+a_2)}) \\ 0 & 0 & 0 & t(1+e^{ik.a_1}) & t_0 & t(1+e^{-ik.a_2}) \\ 0 & 0 & 0 & t(1+e^{ik.(a_1+a_2)}) & t(1+e^{ik.a_2}) & t_0 \\ t_0 & t(1+e^{-ik.a_1}) & t(1+e^{-ik.(a_1+a_2)}) & 0 & 0 & 0 \\ t(1+e^{ik.a_1}) & t_0 & t(1+e^{-ik.a_2}) & 0 & 0 & 0 \\ t(1+e^{ik.(a_1+a_2)}) & t(1+e^{ik.a_2}) & t_0 & 0 & 0 & 0 \end{bmatrix}$$

where $c_{i,D(L)}$ represents destruction operator for an electron at the dark-colored $i^{th}$ atomic site with i being the corresponding site on Kagome lattice, as shown in Fig. 2. It can be clearly seen that the Hamiltonian is chiral symmetric with two copies of Kagome Hamiltonian in off-diagonal blocks. The only addition is the diagonal matrix element in each block, $t_0$ that represents the nearest neighbor hopping between the individual dark and light-colored sites.

d) Bipartite double cover of Kagome lattice (with SOC, single spin channel) –

$$
\begin{array}{cccccc}
c^{\dagger}_{1,D\uparrow} & c^{\dagger}_{2,D\uparrow} & c^{\dagger}_{3,D\uparrow} & c^{\dagger}_{1,L\uparrow} & c^{\dagger}_{2,L\uparrow} & c^{\dagger}_{3,L\uparrow}
\end{array}
$$

$$
\begin{bmatrix}
0 & -i\lambda & i\lambda & t_0 & t(1+e^{-ik.a_1}) & t(1+e^{-ik.(a_1+a_2)}) \\
i\lambda & 0 & -i\lambda & t(1+e^{ik.a_1}) & t_0 & t(1+e^{-ik.a_2}) \\
-i\lambda & i\lambda & 0 & t(1+e^{ik.(a_1+a_2)}) & t(1+e^{ik.a_2}) & t_0 \\
t_0 & t(1+e^{-ik.a_1}) & t(1+e^{-ik.(a_1+a_2)}) & 0 & -i\lambda & i\lambda \\
t(1+e^{ik.a_1}) & t_0 & t(1+e^{-ik.a_2}) & i\lambda & 0 & -i\lambda \\
t(1+e^{ik.(a_1+a_2)}) & t(1+e^{ik.a_2}) & t_0 & -i\lambda & i\lambda & 0
\end{bmatrix}
$$

where $\lambda$ is the SOC strength. We only show one spin-channel here since similar to the case of b), there are no matrix elements between spin-up and spin-down states. The other spin channel can be straightforwardly constructed from $H(k) = H_{L(H)}(k) \otimes \sigma_0 + H_{SOC}(k) \otimes \sigma_z$. Similar to the case of Kagome lattice, we do finite size calculation and observe edge states corresponding to both FBs as shown in Fig. S2(b) confirming the stable topology of the FBs.

e) Kagome-3 lattice (spinless) –

$$
\begin{array}{ccc}
c^{\dagger}_{1} & c^{\dagger}_{2} & c^{\dagger}_{3}
\end{array}
$$

$$
H(L(T)) = \begin{bmatrix}
t(e^{ik.a_2}+e^{-ik.a_2}) & t(1+e^{-ik.a_1})+t(e^{-ik.(a_1+a_2)}+e^{ik.a_2}) & t(1+e^{-ik.(a_1+a_2)})+t(e^{-ik.a_1}+e^{-ik.a_2}) \\
t(1+e^{ik.a_1})+t(e^{ik.(a_1+a_2)}+e^{-ik.a_2}) & t(e^{ik.(a_1+a_2)}+e^{-ik.(a_1+a_2)}) & t(1+e^{-ik.a_2})+t(e^{ik.a_1}+e^{-i(a_1+a_2)}) \\
t(1+e^{ik.(a_1+a_2)})+t(e^{ik.a_1}+e^{ik.a_2}) & t(1+e^{ik.a_2})+t(e^{-ik.a_1}+e^{i(a_1+a_2)}) & t(e^{ik.a_1}+e^{-ik.a_1})
\end{bmatrix}
$$

where the basis set consists of three atomic sites as labelled in Fig. S3(a), and $a_i$'s are unit-cell vectors depicted in Fig. S3(a). The band structure consisting of two exact FBs is reproduced in Fig. S3(b).

f) Kagome-3 lattice with extra s-band (spinless) –

$$
H(L(T)_s) =
$$

$$
\begin{array}{cccc}
c^{\dagger}_{s} & c^{\dagger}_{1} & c^{\dagger}_{2} & c^{\dagger}_{3}
\end{array}
$$

$$
\begin{bmatrix}
\mathbf{t_s^2} & \mathbf{t_s(1+e^{ik.a_2})} & \mathbf{t_s(e^{ik.a_2}+e^{-ik.a_1})} & \mathbf{t_s(1+e^{-ik.a_1})} \\
\mathbf{t_s(1+e^{-ik.a_2})} & t(e^{ik.a_2}+e^{-ik.a_2}) & t(1+e^{-ik.a_1})+t(e^{-ik.(a_1+a_2)}+e^{ik.a_2} & t(1+e^{-ik.(a_1+a_2)})+t(e^{-ik.a_1}+e^{-ik.a_2}) \\
\mathbf{t_s(e^{-ik.a_2}+e^{ik.a_1})} & t(1+e^{ik.a_1})+t(e^{ik.(a_1+a_2)}+e^{-ik.a_2}) & t(e^{ik.(a_1+a_2)}+e^{-ik.(a_1+a_2)}) & t(1+e^{-ik.a_2})+t(e^{ik.a_1}+e^{-i(a_1+a_2)}) \\
\mathbf{t_s(1+e^{ik.a_1})} & t(1+e^{ik.(a_1+a_2)})+t(e^{ik.a_1}+e^{ik.a_2}) & t(1+e^{ik.a_2})+t(e^{-ik.a_1}+e^{i(a_1+a_2)}) & t(e^{ik.a_1}+e^{-ik.a_1})
\end{bmatrix}
$$

where in addition to the three atomic sites in e), there is an additional site in the unit cell indicated by dashed red circle in Fig. 4(a) and in Fig. S3(a). $t_s$ indicates nearest-neighbor hopping integral between the additional s-site and the remaining sites in the unit-cell. Hence, the Hamiltonian consists of Kagome-3 matrix block (same as in e)) with extra row and column (indicated in red) corresponding to $c^{\dagger}_{s}$, operator that creates electron at atomic site s. Note that the onsite energy of extra orbital is arbitrarily set to $t_s^2$ without loss of generality. At $t_s = 3t$, the band structure consists of 2 fragile exact FBs, a trivial band near the FBs and another dispersive band far away from the set of 3 bands as shown in Fig. S3(c).

g) Bipartite double cover of Kagome-3 lattice (spinless) –

$$
\begin{array}{cc}
\{c^{\dagger}_{1D}, c^{\dagger}_{2D}, c^{\dagger}_{3D}\} & \{c^{\dagger}_{1L}, c^{\dagger}_{2L}, c^{\dagger}_{3L}\}
\end{array}
$$

$$
H\Big(B\big(L(T)\big)\Big) = \begin{bmatrix}
0 & H\big(L(T)\big) + t_0 I \\
H\big(L(T)\big) + t_0 I & 0
\end{bmatrix}
$$

where similar to c) the chiral symmetric bipartite double cover can be constructed by simply placing the Kagome-3 Hamiltonian at off-diagonal blocks. $t_0$ represents intra-hopping of individual dark-light atomic sites as depicted in Fig. 4(c).

h) Bipartite double cover of Kagome-3 lattice with extra s-band (spinless) –

$$H\big(B(L(T))\big) = \begin{matrix} \{c_{sD}^\dagger, c_{1D}^\dagger, c_{2D}^\dagger, c_{3D}^\dagger\} & \{c_{sL}^\dagger, c_{1L}^\dagger, c_{2L}^\dagger, c_{3L}^\dagger\} \\ \end{matrix} \begin{bmatrix} 0 & H(L(T)_s) + t_0 I \\ H(L(T)_s) + t_0 I & 0 \end{bmatrix}$$

The band structure corresponding to this Hamiltonian is shown in Fig. S4(a) at $t_s = 3t$ and $t_0 = 2t$.

i) $sp^2$ orbitals on hexagonal lattice (with SOC, single spin channel) –

$$H = \begin{matrix} \{c_{s,A}^\dagger, c_{p_x,A}^\dagger, c_{p_y,A}^\dagger\} & \{c_{s,B}^\dagger, c_{p_x,B}^\dagger, c_{p_y,B}^\dagger\} \end{matrix} \begin{bmatrix} H_{SOC} & H' \\ H'^\dagger & H_{SOC} \end{bmatrix}$$

with the block matrices given by –

$$H_{SOC} = \begin{bmatrix} 0 & 0 & 0 \\ 0 & 0 & i\lambda \\ 0 & -i\lambda & 0 \end{bmatrix},$$

$$H' = \begin{bmatrix} t_{ss\sigma}\left(e^{ik_2} + e^{i(k_1+k_2)} + e^{ik_1}\right) & t_{sp\sigma}\left(\frac{\sqrt{3}}{2}\right)\left(e^{ik_2} - e^{i(k_1+k_2)}\right) & t_{sp\sigma}\left(\frac{1}{2}\right)\left(-e^{ik_2} - e^{i(k_1+k_2)} + 2e^{ik_1}\right) \\ t_{sp\sigma}\left(\frac{\sqrt{3}}{2}\right)\left(-e^{ik_2} + e^{i(k_1+k_2)}\right) & t_{pp\pi}e^{ik_1} + \left(-\frac{3t_{pp\sigma}}{4} + \frac{t_{pp\pi}}{4}\right)\left(e^{ik_2} + e^{i(k_1+k_2)}\right) & (t_{pp\sigma} + t_{pp\pi})\left(\frac{\sqrt{3}}{4}\right)\left(e^{ik_2} - e^{i(k_1+k_2)}\right) \\ t_{sp\sigma}\left(\frac{1}{2}\right)\left(e^{ik_2} - 2e^{i(k_1+k_2)} + e^{ik_1}\right) & (t_{pp\sigma} + t_{pp\pi})\left(\frac{\sqrt{3}}{4}\right)\left(e^{ik_2} - e^{i(k_1+k_2)}\right) & -t_{pp\sigma}e^{ik_1} + \left(-\frac{t_{pp\sigma}}{4} + \frac{3t_{pp\pi}}{4}\right)\left(e^{ik_2} + e^{i(k_1+k_2)}\right) \end{bmatrix}$$

where $k_i = k.a_i$ with $a_i$ being the lattice vectors of hexagonal lattice with A and B sublattices labelled in Fig. S5. The other spin channel can be directly written with $\lambda \to -\lambda$.

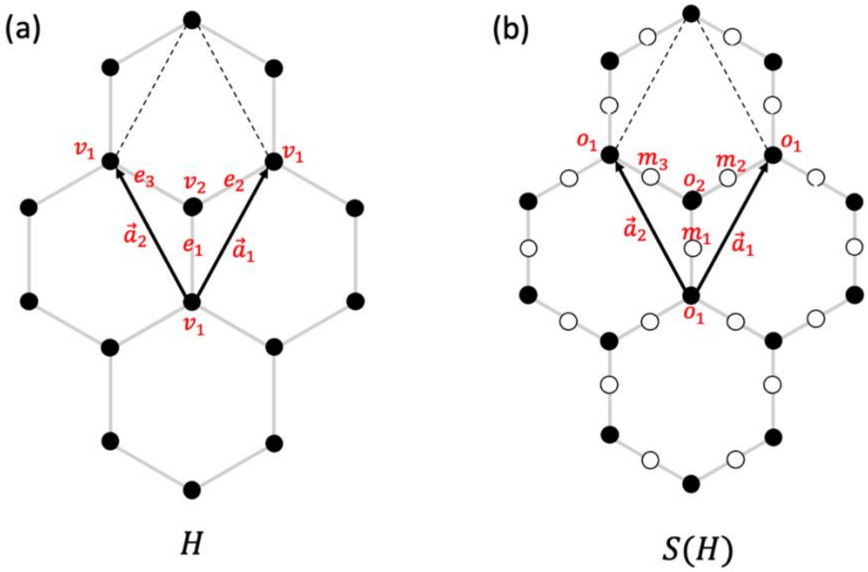


Fig. S1. (a) Honeycomb Lattice - $\vec{a}_i$ denote the lattice vectors, $e_i$ and $v_i$ are the independent edges and vertices in the unit cell. (b) Square root of honeycomb lattice – black circles denote the original sites ($o_i$), while the white circles indicate the mediating sites ($m_i$).

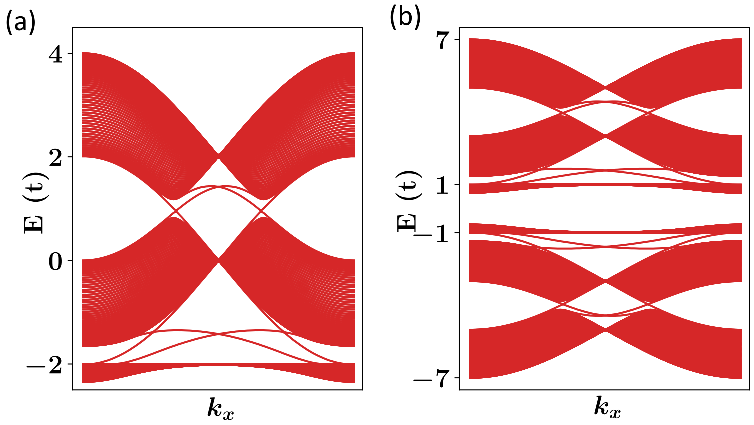


Fig. S2. Band structure of the finite size (60 unit cells) Kagome lattice ((a)), and its bipartite double cover ((b)) in y-direction.

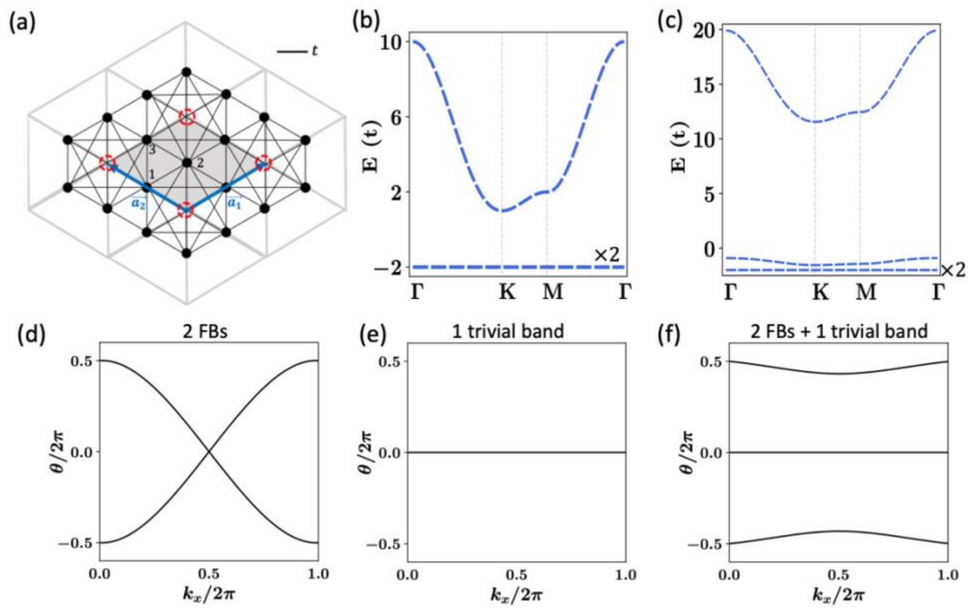


Fig. S3. (a) Line-graph of triangular lattice – Kagome-3 lattice. (b) Two exact FBs at $\mathrm{E} = -2\mathrm{t}$ in the band structure of the line-graph lattice of triangular lattice, Kagome-3. (c) Electronic band structure of Kagome-3 lattice with an additional s-orbital at Wycoff position as indicated in (a). Hopping parameter, $\mathrm{t_s} = 3\mathrm{t}$. (d) Wilson loop spectra for the two FBs in (a). Winding in the spectra is indicative of non-trivial topology. (e) Wilson loop spectra of the extra band near the two FBs in (b). This band is trivial. (f) Wilson loop spectra of three bands (two FBs and additional s-band) in (b). The winding of the two FBs is removed by the addition of a trivial band demonstrating that the FBs are fragile topological.

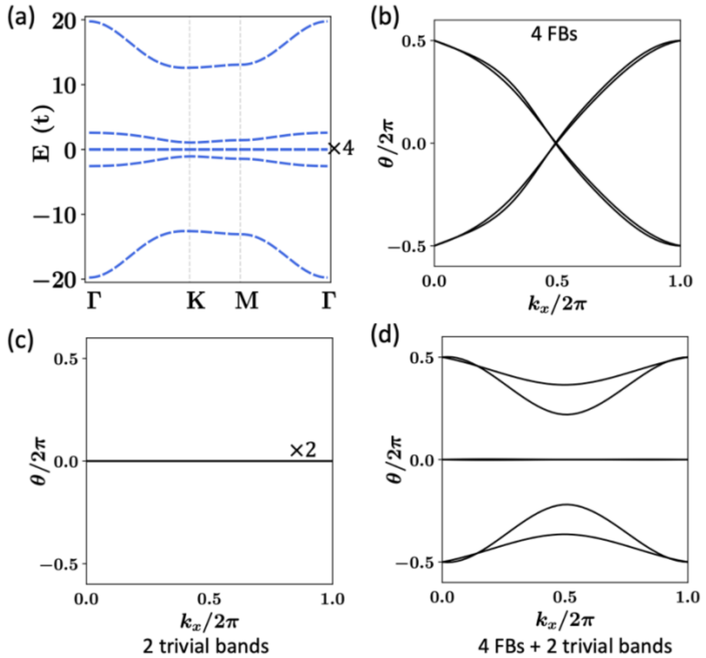


Fig. S4. (a) Band structure of the bipartite double cover of Kagome-3 with additional s- orbital consisting of bonding and anti-bonding pairing of the bands in Fig. S2(b). (b) Wilson loop spectra of

the four exact FBs at charge neutrality in (a). The two sets of FBs have non-trivial winding. (c) Wilson loop spectra of the two s-bands near charge neutrality in (a). These bands are trivial. (d) Wilson loop spectra of six bands in (b) and (c) together. Non-trivial winding of the FBs is removed by the addition of trivial bands confirming fragile topology of the FBs.

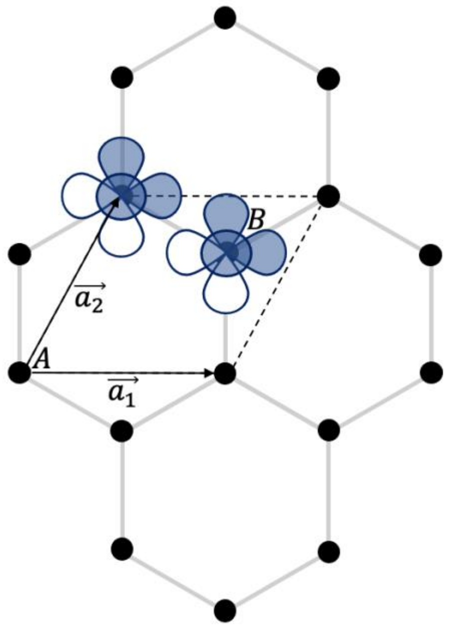


Fig. S5. $sp^2$-orbitals on hexagonal lattice.

## III. Wilson Loop Analysis:

In order to confirm the fragile topology of exact FBs in Kagome-3 lattice and its bipartite double cover, we do Wilson loop analysis using Wilson loop operator [9,10]. Consider a Hamiltonian $\mathrm{H(k)}$ consisting of two occupied bands with wavefunctions $\mathrm{u_{0k}}$, and $\mathrm{u_{1k}}$ calculated in unit-cell gauge. One can construct an $\mathrm{m} \times 2$ matrix of the occupied bands $\mathrm{U_k} = [\mathrm{u_{0k}}; \mathrm{u_{1k}}]$ where m is the number of sites in the unit-cell. The Wilson loop can be calculated along reciprocal lattice vectors with reciprocal momenta parametrized as $\mathrm{k} = \mathrm{k_1 b_1} + \mathrm{k_2 b_2}$ where $\mathrm{k_j} \in [0,1]$ and $\mathrm{b_j}$'s are the reciprocal lattice vectors. The discretized Wilson loop integrated along $\mathrm{k_2}$ is then given by –

$$\mathrm{W(k_1)} = \mathrm{U^{\dagger}_{k_1,0} U_{k_1,\frac{1}{N}} U^{\dagger}_{k_1,\frac{1}{N}} U_{k_1,\frac{2}{N}} \cdots U^{\dagger}_{k_1,\frac{N-1}{N}} U_{k_1,0}},$$

where N is the number of discretized k-points along $\mathrm{k_1}$. Next, to ensure unitarity of $\mathrm{W(k_1)}$, a singular value decomposition is done using –

$$\mathrm{G_{k_1,\frac{j}{N}}} = \mathrm{U^{\dagger}_{k_1,\frac{j}{N}} U_{k_1,\frac{j+1}{N}}} = \mathrm{SDP^{\dagger}},$$

with D being the diagonal matrix. Wilson operator can then be defined in terms of the matrix $\mathrm{F_{k_1,\frac{j}{N}}} = \mathrm{SP^{\dagger}}$ -

$$W(k_1) = F_{k_1,0}F_{k_1,\frac{1}{N}} \dots F_{k_1,\frac{N-1}{N}}F_{k_1,0}.$$

This Wilson operator is unitary and can be expressed as $W(k_1) = e^{iH_w(k_1)}$. Hence the Wilson Hamiltonian is given by –

$$H_W(k) = -i\log W(k_1).$$

For two FBs of Kagome-3 lattice this would be a $2 \times 2$ Hermitian matrix that can be solved to get the Wilson spectra as plotted in Fig. S3(d). The two FBs have non-trivial and opposite winding, indicative of its non-trivial topology. Similarly, we calculate the Wilson spectra for the three lowest bands of Hamiltonian described in II. f) where an additional band is introduced in Kagome-3 lattice. For this extra band alone, the Wilson loop shows no winding implying that the extra band is trivial (Fig. S3(e)). On the other hand, if the three bands are considered together, the winding of even the two FBs is destroyed as shown in Fig. S3(f). This clearly illustrates the fragile topology of the FBs since the topological obstruction to Wannier localization is resolved by the addition of a trivial band. Similar analysis can be done for the four FBs of bipartite double cover of Kagome-3 lattice as described in the main text and in Fig. S4.

## IV. Additional examples of 2D and 3D line-graph lattices and their bipartite double covers:

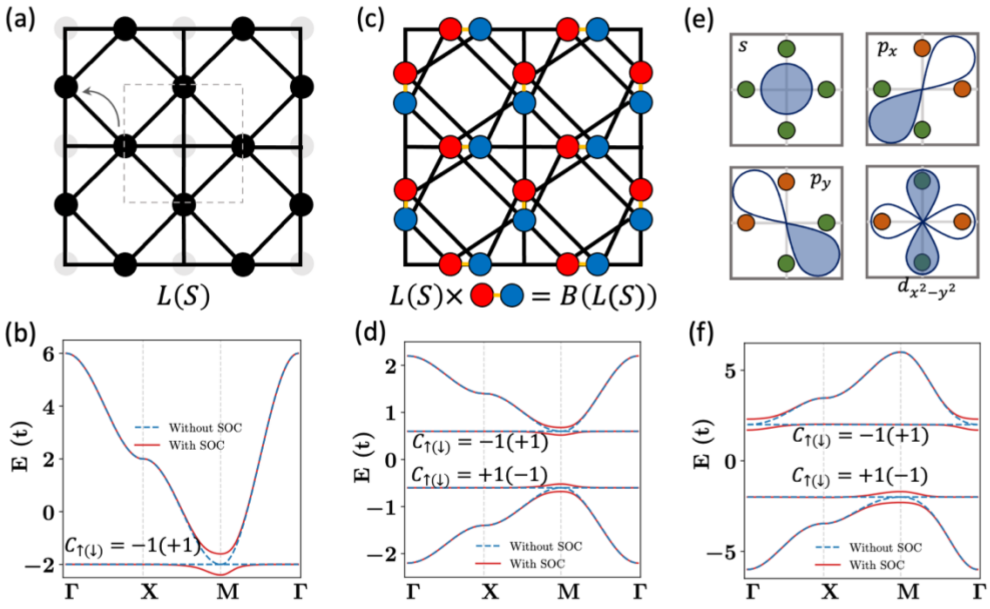


Fig. S6. (a) Line-graph of 2D square lattice - 2D Checkerboard lattice. Unit cell is marked with dashed square box. (b) Electronic band structure of (a) with a FB at $E = -2t$. SOC is included by adding positive (negative) imaginary hopping terms in (opposite to) the direction indicated by arrow in (a). (c) Bipartite double cover construction of (a). (d) Band structure of (c) with Hamiltonian constructed using Eqn. 2 forming a quantum semiconductor with flat valence and conduction bands of opposite chirality. (e) Orbital design using symmetries of the Γ-point wavefunctions of the four bands in (d). (f) Band structure obtained using Slatter-Koster integrals for $sp^2d$ orbitals on square lattice.

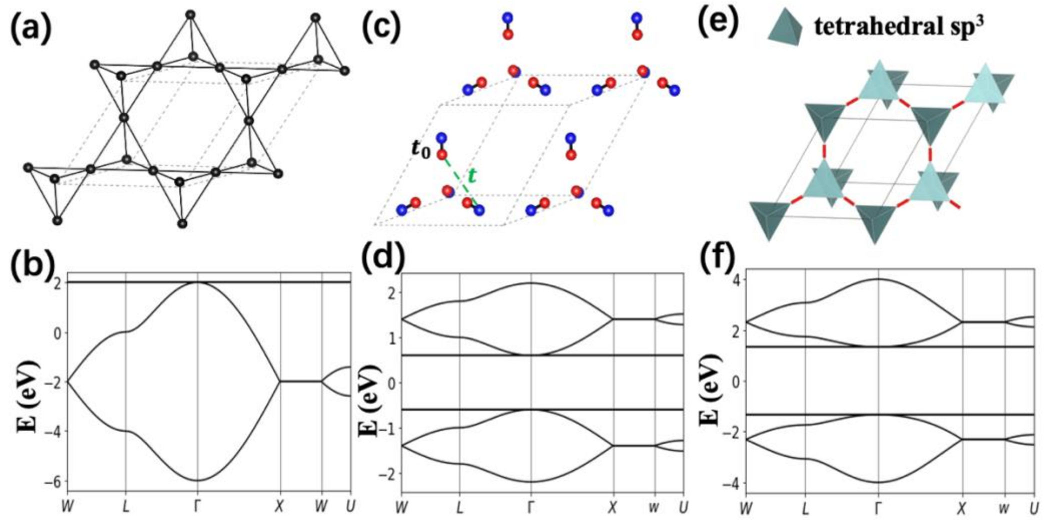


Fig. S7. Yin-yang FBs in a 3D lattice. (a) Pyrochlore lattice [11]. (b) The band structure of pyrochlore lattice. (c) Bipartite double cover of pyrochlore lattice. Two sublattice sites are denoted by red and blue balls, respectively. First nearest-neighbor hopping $t_0$ and BDC graph hopping $t$ are marked by black solid lines and green dashed lines, respectively. (d) The band structure of 3D yin-yang FB plotted at $t = 1/3t_0$. (e) $sp^3$ diamond lattice. Each tetrahedron represents four $sp^3$ orbitals on diamond lattice sites. (f) The band structure of $sp^3$ diamond lattice.

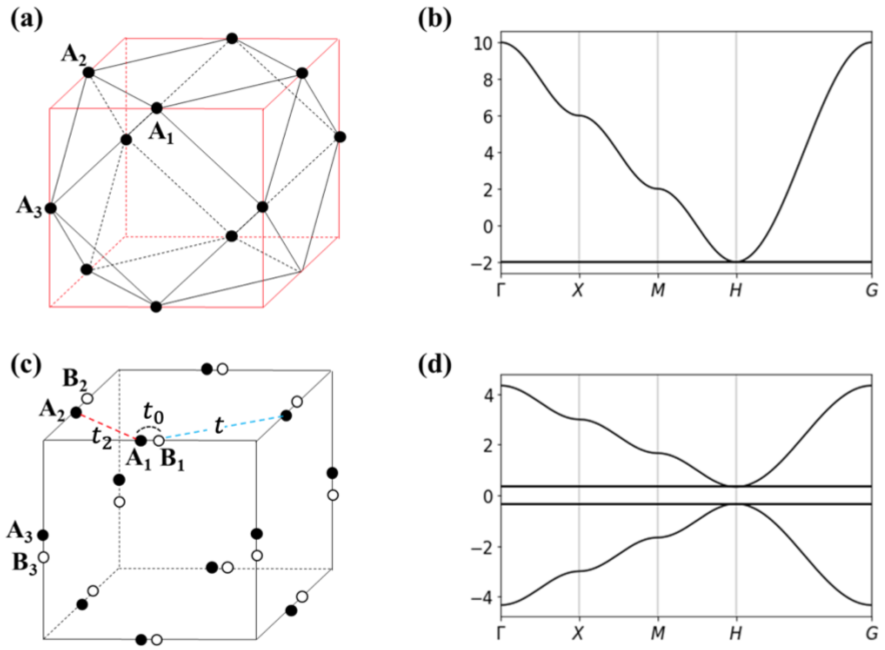


Fig. S8. (a) Unit cell of 3D checkerboard lattice. (b) The band structure of 3D checkerboard lattice. (c) Bipartite double cover of 3D twin checkerboard lattice with $t_0$ being the first nearest-neighbor hopping, $t$ being the BDC graph hopping, and $t_2$ denoting the $2^{nd}$ nearest-neighbor hopping integral. The two

BDC sublattices are indicated by $A_i$ and $B_i$. (d) The 3D yin-yang FBs of 3D twin checkerboard lattice with hopping integrals $t_0 = 1$ eV, $t_2 = 0, t = 1/3t_0$.

## References


[1] Cvetkovic, D. M., Doob, M., & Sachs, H. (1980). Spectra of graphs. Theory and application. Academic Press.

[2] Biggs, N. (1993). Algebraic graph theory (No. 67). Cambridge university press.

[3] Kollár, A. J., Fitzpatrick, M., Sarnak, P., & Houck, A. A. (2020). Line-graph lattices: Euclidean and non-Euclidean flat bands, and implementations in circuit quantum electrodynamics. Communications in Mathematical Physics, 376, 1909-1956.

[4] Arkinstall, J., Teimourpour, M. H., Feng, L., El-Ganainy, R., & Schomerus, H. (2017). Topological tight-binding models from nontrivial square roots. Physical Review B, 95(16), 165109.

[5] Ezawa, M. (2020). Systematic construction of square-root topological insulators and superconductors. Physical Review Research, 2(3), 033397.

[6] Mizoguchi, T., Yoshida, T., & Hatsugai, Y. (2021). Square-root topological semimetals. Physical Review B, 103(4), 045136.

[7] Liu, H., Sethi, G., Meng, S., & Liu, F. (2022). Orbital design of flat bands in non-line-graph lattices via line-graph wave functions. Physical Review B, 105(8), 085128.

[8] Song, Z. D., Elcoro, L., & Bernevig, B. A. (2020). Twisted bulk-boundary correspondence of fragile topology. Science, 367(6479), 794-797.

[9] Alexandradinata, A., Dai, X., & Bernevig, B. A. (2014). Wilson-loop characterization of inversion-symmetric topological insulators. Physical Review B, 89(15), 155114.

[10] Peri, V., Song, Z. D., Bernevig, B. A., & Huber, S. D. (2021). Fragile topology and flat-band superconductivity in the strong-coupling regime. Physical review letters, 126(2), 027002.

[11] Zhou, Y., Jin, K. H., Huang, H., Wang, Z., & Liu, F. (2019). Weyl points created by a three-dimensional flat band. Physical Review B, 99(20), 201105.
